# Supplementary material for: Challenges in Measuring Transport Parameters of Carbonate-based Electrolytes
Source: arXiv:2401.09173 ancillary file (2024-01-17)
Supplement: Supplementary file 1 [file main_supp.pdf]

# Supporting Information: Challenges in Measuring Transport Parameters of Carbonate-based Electrolytes

Lukas Lehnert, Maryam Nojabaee, Arnulf Latz, Birger Horstmann

## Contents

**1. Cell Constant $k$ and Additional Conductivity Cell Measurements** **1**

**2. Additional Concentration Cell Measurements** **1**

**3. Galvanostatic Polarization Experiments** **2**
3.1. Determination of $R_{\mathrm{el}}$, $R_{\mathrm{int}}$ and $\beta$ Using EIS . . . 2
3.2. Non-Linearities . . . 3
3.3. Determination of $U_{\mathrm{c}}$ . . . 3
3.4. Determination of $D_{\pm}(c_0)$ . . . 4

**4. Very-Low-Frequency Impedance Spectroscopy** **5**
4.1. Non-Linearities . . . 5
4.2. Drift Correction . . . 8
4.3. Determination of $R_{\mathrm{el}}$, $R_{\mathrm{int}}$ and $\beta$ . . . 8
4.4. Concentration Gradient Dependence of $R_{\mathrm{D}}^{\mathrm{tot}}$ . . . 9
4.5. Distribution of Relaxation Times (DRT) . . . 10
4.6. Fast Growing Porous Layers on the Li Electrodes . . . 11

## 1. Cell Constant $k$ and Additional Conductivity Cell Measurements

In section 3.1 the authors measure the impedance of the sole 0.5 M $LiPF_6$ in EC:EMC (3:7, weight) electrolyte using conductivity cells. Translating the electrolyte resistance $R_{\mathrm{el}}$ to the corresponding conductivity requires the cell constant $k$ (see Eq. 29). Measuring the impedance of a reference electrolyte with known conductivity $\kappa$ enables specifying $k$.
Evaluating the EIS measurement of the reference electrolyte (Conductivity Standard ROTI®Calipure 12880 µS/cm (25 °C)) yields $k = 19.7 \pm 0.2\,\frac{1}{\mathrm{cm}}$ at 20 °C and $k = 16.18 \pm 0.01\,\frac{1}{\mathrm{cm}}$ at 50 °C for the cell constant. This discrepancy probably originates from polishing the platinum electrodes after finishing all measurements at 20 °C, as the cell constant does not significantly change with temperature.
In the course of the conductivity measurements, we determined the conductivity of $LiPF_6$ in EC:EMC (3:7, weight) for various concentrations and temperatures with the same set-up described in section 2.2.1. For completeness, Figure 1 shows them here. The data exhibits good agreement with the literature.[1] Note that at -30 °C, the electrolyte might form solid crystals.

## 2. Additional Concentration Cell Measurements

We conducted additional concentration cell measurements for various base concentrations of $LiPF_6$ in EC:EMC (3:7, weight) and at different temperatures with the same set-up described in section 2.2.2. The data (see Figure 2) shows good agreement with the

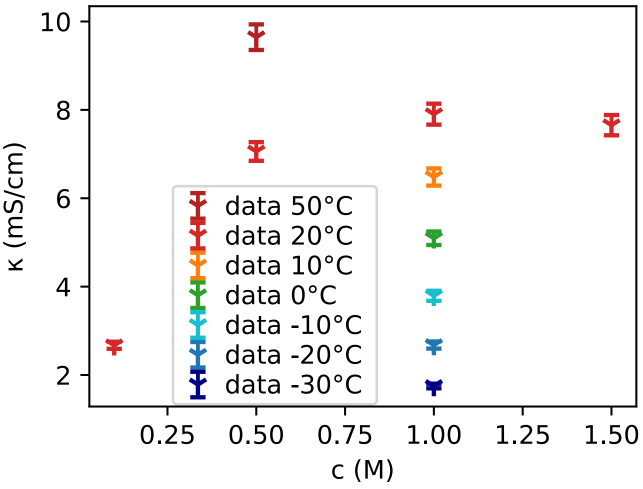


**Figure 1.** Additional conductivity measurements for various concentrations and temperatures.

literature.[1] As explained in Section 2.3, the evaluation of the concentration cell data of this system using Newman's concentrated solution theory[2] deviates from the evaluation using the theory from Latz et al.[3,4] by a factor of 2. At -30 °C, the electrolyte might form solid crystals.

# 3. Galvanostatic Polarization Experiments

## 3.1. Determination of $R_{el}$, $R_{int}$ and $\beta$ Using EIS

In order to determine the diffusion coefficient $D_{\pm}(c_0)$ and factor $b(c_0)$ the authors apply galvanostatic polarization experiments to symmetrical Li metal | electrolyte + separator | Li metal cells and measure the corresponding potential response $\Delta\Phi$. The morphology of the separator influences the behavior of $\Delta\Phi$. Therefore, the identification of $D_{\pm}(c_0)$ and $b(c_0)$ of the sole electrolyte requires specifying the Bruggemann-coefficient $\beta$ of the separator ($\varepsilon$ is stated by the manufacturer, see section 2.2.3). For this, we conduct potentiostatic EIS measurements between every polarization experiment from 4 MHz down to 1 Hz with an amplitude of 5 mV yielding the bulk resistance $R_{el}$ and the interface resistance $R_{int}$. Inserting $R_{el}$ and the measured conductivity $\kappa(c_0)$ (see section 3.1) in Eq. 23 reveals the Bruggemann-coefficient $\beta$.

In the Nyquist-plot, the shape of each EIS measurement at both temperatures is similar. At high frequencies, the real part of the EIS data shows an offset corresponding to the bulk resistance of the electrolyte-separator system. This offset is followed by a depressed arc induced by the SEI, charge-transfer and double-layer effects.

For fitting the impedance spectra we use the RealxIS software (rhd instruments) and the equivalent circuit shown in Figure 3. A serial resistance represents the bulk resistance $R_{el}$. Two additional R-CPE elements incorporate the impedance of the SEI and the charge transfer and double layer effects. For simplification, these effects are summarized in the interface resistance $R_{int}$ since $R_{el}$ is of main interest.

For both temperatures, $R_{el}$ slightly increases from measurement to measurement for all three cells, except for one cell at 20 °C (see Figure 4a). Using the respective mean value yields a Bruggemann-coefficient of $\beta = 2.72 \pm 0.09$ and $\beta = 2.5 \pm 0.1$ at 20 °C and 50 °. This is in good agreement with the values measured by Landesfeind et al.[5] for a similar electrolyte at 25 °C.

The interface resistance $R_{int}$ stays rather stable from measurement to measurement at 20 °C. At 50 °C, it slowly decreases (see Figure 4b).

As mentioned in section 3.3 the growth of an additional porous layer consisting of live and dead mossy Li allows explaining the trends of $R_{el}$ and $R_{int}$.[6] Additional dead mossy Li increases the bulk resistance which could

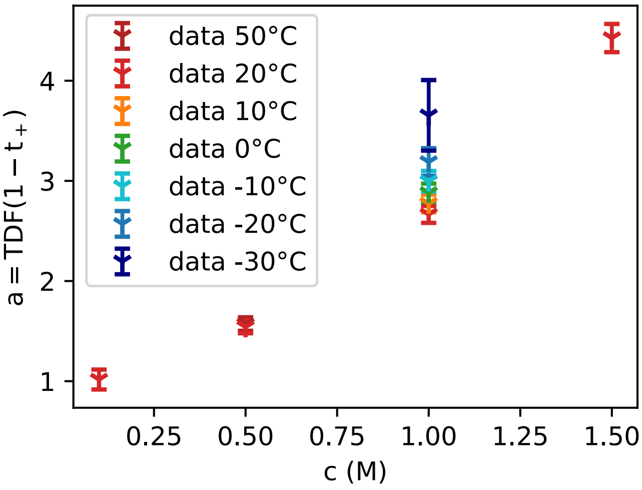


**Figure 2.** Additional concentration cell measurements for various concentrations and temperatures.

explain the increase of $R_{el}$ in our impedance measurements (see Figure 4a). Depending on the amount of dead mossy Li, calculating the Bruggemann-coefficient $\beta$ with Eq. 23 may hence overestimate its actual average value. However, the increase of $R_{el}$ does not correlate with the total transferred charge. Note, that the current amplitude in our polarization experiments changes according to Table 2. Therefore, the effect could also originate from electrolyte degradation. However, diminishing the solution phase would increase the concentration of the electrolyte and therefore increase its conductivity, leading to smaller resistances.

Covering the pristine Li electrode with live mossy Li increases the active electrode area, leading to elevated reaction kinetics. Thus the interface resistances $R_{int}$ decreases. On the other hand, a growing SEI induces increasing $R_{int}$ values. Therefore, there are two possible ways to explain the constant $R_{int}$ at 20 °C (see Figure 4b). Either, the cells show almost no growth of SEI or live Li. Or both competing effects cancel each other out. At 50 °C, $R_{int}$ decreases. Hence, the influence of growing live mossy Li coverage seems to surpass the effects of the possibly growing SEI. However, also the decrease in $R_{int}$ does again not correlate

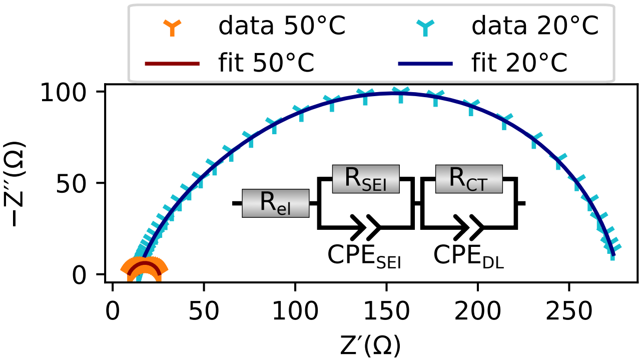


**Figure 3.** Exemplary EIS data at 20 °C and 50 °C conducted between the polarization experiments. We fit the data using the shown equivalent circuit.

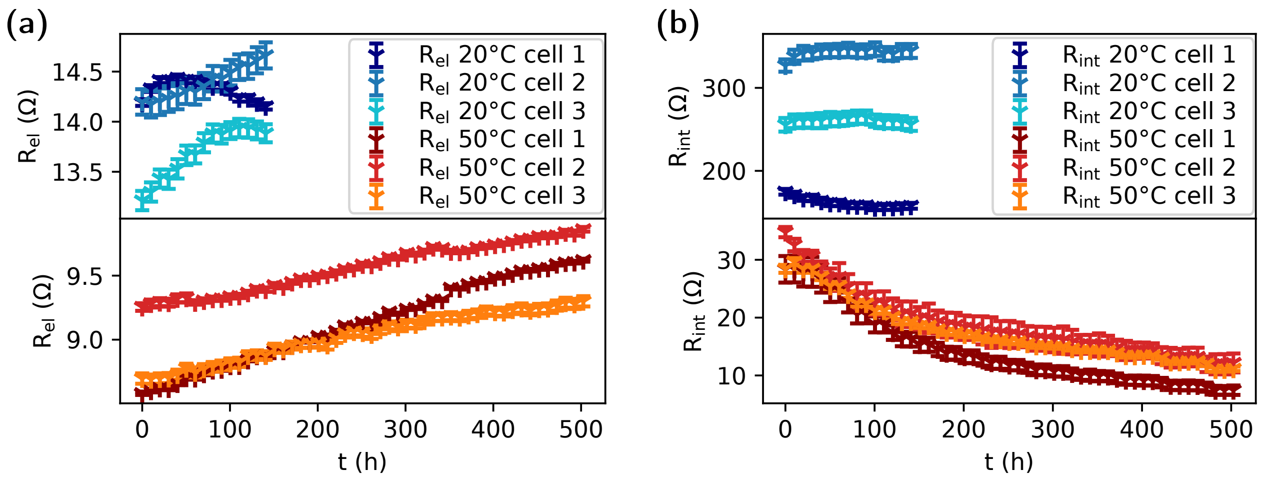


**Figure 4. a)** Bulk resistance $R_{\mathrm{el}}$ of the electrolyte-separator system. At both temperatures, $R_{\mathrm{el}}$ shows mainly increasing trends, except for one cell at 20 °C. **b)** Interface resistance $R_{\mathrm{int}}$. At 20 °C, $R_{\mathrm{int}}$ exhibits stable behavior. At 50 °C, $R_{\mathrm{int}}$ decreases. For both plots, the error bars account for the fit error.

with the total transferred charge.

## 3.2. Non-Linearities

In our galvanostatic polarization experiments, the authors apply high current densities to induce significantly high concentration gradients $\Delta c$. These amplitudes could induce non-linear effects. Therefore, we use our 1D-model (see section 2.3) to check the validity of our linear response theory.
The procedure is quite equal to the non-linearity check for our VLF-IS measurements conducted with the same current amplitudes (see section 4.1). In the VLF-IS, the lowest frequencies induce similar concentration gradients $\Delta c$ as the polarization experiments and thus similar non-linearities. Therefore, we refer the reader for details to section 4.1. Figure 5 exemplary shows the potential response $\Delta\Phi$ of the simulated galvanostatic polarization experiments with the highest current amplitudes $I_0 = 60\,\mu\mathrm{A}$ and $I_0 = 500\,\mu\mathrm{A}$ at both temperatures. Comparing these potentials to a by a factor 12 and 100 up-scaled respective linear reference with $I_0 = 5\,\mu\mathrm{A}$ yields nearly no deviation at each temperature, respectively. Therefore, non-linear contributions are negligibly small.

## 3.3. Determination of $U_{\mathrm{c}}$

The charging process of the galvanostatic polarization experiments establishes a concentration gradient $\Delta c$. For long charging times, the concentration profile becomes linear and induces the concentration potential $U_{\mathrm{c}}$ (see section 2.1.2). To determine $U_{\mathrm{c}}$ the authors calculate $U_{\bar{i}} = (R_{\mathrm{el}} + R_{\mathrm{int}})\, I_0$ using the impedance measurements before and after the corresponding polarization experiment. Measuring the steady-state potential $\Delta\Phi$ right before the current interruption time $T_{\mathrm{I}}$ and subtracting $U_{\bar{i}}$ (see Figure 1a) yields $U_{\mathrm{c}} = \Delta\Phi\,(t = 1\,\mathrm{h}) -$

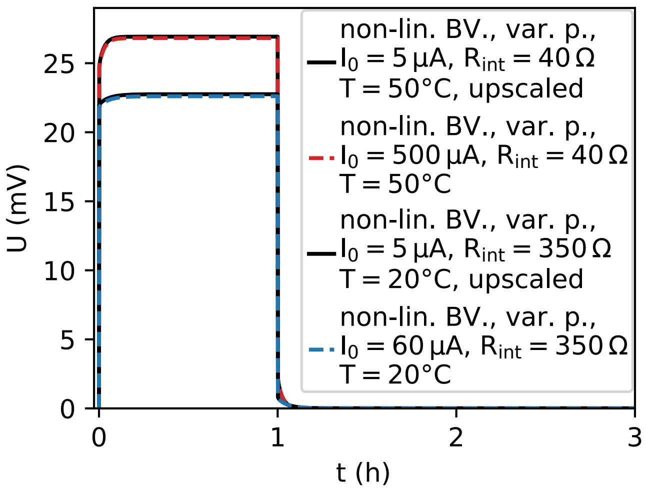


**Figure 5.** Simulated polarization experiments at 20 °C and 50 °C. The potential responses for the highest current amplitudes $I_0 = 60\,\mu\mathrm{A}$ and $I_0 = 500\,\mu\mathrm{A}$ compare to the respective up-scaled linear reference with $I_0 = 5\,\mu\mathrm{A}$. At both temperatures, the comparison yields hardly any difference indicating negligible non-linear contributions.

$U_{\bar{i}}$. We average this value with the corresponding potential $U_{\mathrm{c}} = \Delta\Phi\,(t = T_{\mathrm{I}} + \delta t)$ measured directly after the current interruption time $T_{\mathrm{I}}$.
To facilitate the comparison of $U_{\mathrm{c}}$ for the various applied current densities Figure 6b shows $R_{\mathrm{c}} = \frac{U_{\mathrm{c}}}{I_0}$. However, instead of exhibiting nearly constant values $R_{\mathrm{c}}$ decreases with increasing concentration gradient $\Delta c$ at both temperatures. To ensure that the decrease of $R_{\mathrm{c}}$ is not only a time-dependent phenomenon we analyze the $I_0 = 10\,\mu\mathrm{A}$ reference measurements conducted between the polarization experiments with increasing $I_0$ at 50 °C (see Table 2). In these reference experiments, $R_{\mathrm{c}}$ in fact shows a slight decreasing trend over time for the first half of the measurements. For longer times $R_{\mathrm{c}}$ marginally increases. However, compared to a measurement with high $I_0$ the $I_0 = 10\,\mu\mathrm{A}$ reference measurements show significantly higher $R_{\mathrm{c}}$ values for all times

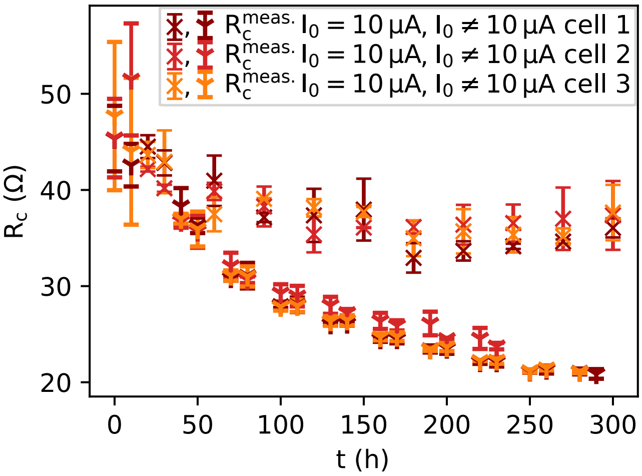


**Figure 6.** Measured $R_c$ over time. $R_c$ varies slightly over time for the $I_0 = 10\,\mu A$ reference measurements. For high $I_0$ $R_c$ decreases compared to the references, indicating a dependency on the concentration gradient $\Delta c$. The error bars represent the respective standard deviation.

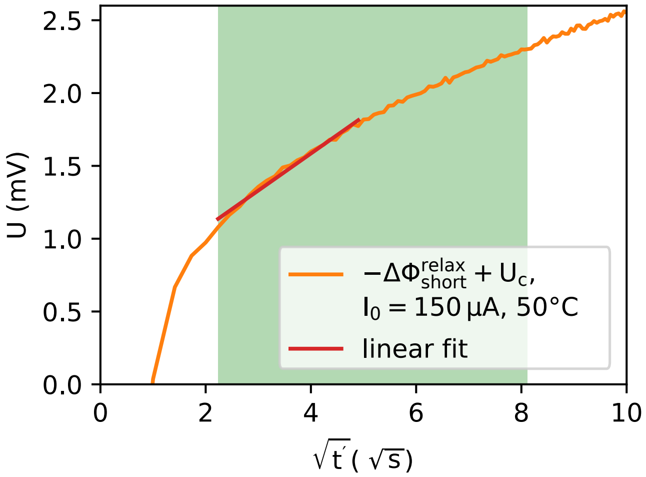


**Figure 7.** Exemplary fit of $-\Delta\Phi_{short}^{relax} + U_c$ over $\sqrt{t'}$. The green area indicates the time within the potential theoretically shows linear behavior. Since the potential exhibits curved behavior, we use 20 s long time intervals for the linear fit. The red line shows an exemplary fit using the time interval which contains the shortest times.

(see Figure 6). This indicates a clear dependence on the concentration gradient $\Delta c$.

## 3.4. Determination of $D_\pm(c_0)$

Evaluating the temporal evolution of the potential response $\Delta\Phi(t)$ in the galvanostatic polarization experiments reveals $D_\pm(c_0)$. For short times $t$ and $t' = t - T_I$ after the current interruption time $T_I$, the terms $\Delta\Phi_{short}^{charge} - U_{\bar{i}}$ and $-\Delta\Phi_{short}^{relax} + U_c$ theoretically exhibit a linear slope $m_{sqrt}$ over $\sqrt{t}$ and $\sqrt{t'}$ respectively. However, as opposed to the theory, the potential shows solely curved behavior (see Figure 7a).
To determine $D_\pm^{sqrt}(c_0)$ we evaluate $\Delta\Phi_{short}^{charge} - U_{\bar{i}}$ and $-\Delta\Phi_{short}^{relax} + U_c$ over $\sqrt{t}$ and $\sqrt{t'}$ within the time interval during which the corresponding simulations yield linear behavior. According to our 1D-model (see section 2.3) the linear slope should be maintained from $t = t' = 0$ s up to $t = t' = 130$ s and $t = t' = 66$ s at 20 °C and 50 °C. For greater times the slope deviates for $> 5\%$ from their linear short-time approximation. To exclude possible measurement artifacts occurring at the beginning of the charging and relaxation processes from the analysis the authors neglect the data of the first 4 s. Since the potential resolution is quite low during the charging process only the relaxation data enters the fitting procedure.
We linearly fit the potential using 20 s long time segments to determine $m_{sqrt}$ (see Figure 7). Inserting $m_{sqrt}$ in Eq. 18 yields $D_\pm^{sqrt}(c_0)$. Due to the curved slope, $D_\pm^{sqrt}(c_0)$ exhibits a range of values in the time interval considered for the evaluation. For the time segments including the longest times, $D_\pm^{sqrt}(c_0)$ shows similar values for all current densities with $D_\pm^{sqrt}(c_0) = (0.9 \pm 0.2) \cdot 10^{-10}\,\frac{m^2}{s}$ at 20 °C and $D_\pm^{sqrt}(c_0) = (2.1 \pm 0.7) \cdot 10^{-10}\,\frac{m^2}{s}$ at 50 °C on average. These values are lower than the literature values.[1] Note, that the signal-to-noise ratio is very low for the measurements with $I_0 = 5\,\mu A$ for these time segments which are therefore excluded from the analysis.
Using earlier time intervals for the fit results in elevated diffusion coefficients. Thus, $D_\pm^{sqrt}(c_0)$ shows the highest values for the time segments including the shortest times. Here, $D_\pm^{sqrt}(c_0)$ depends on the concentration gradient. While the 10 µA reference measurements at 50 °C yield relatively constant values of $D_\pm^{sqrt}(c_0) = (4 \pm 1) \cdot 10^{-10}\,\frac{m^2}{s}$ on average, the diffusion coefficient takes values up to $D_\pm^{sqrt}(c_0) = 5.5 \cdot 10^{-10}\,\frac{m^2}{s}$ for elevated concentration gradients (see Figure 7c). At 20 °C, $D_\pm^{sqrt}(c_0)$ shows varying values over $\Delta c$ from $4.6 \cdot 10^{-10}\,\frac{m^2}{s}$ up to $8.6 \cdot 10^{-10}\,\frac{m^2}{s}$ surpassing the values of $D_\pm^{sqrt}(c_0)$ at 50 °C. This opposes the trend reported by the literature.[1]
For long times $t$ and $t'$, the terms $\ln\left(\Delta\Phi_{long}^{relax}\right)$ and $\ln\left(\Delta\Phi_{long}^{charge} - U_{\bar{i}} - U_c\right)$ theoretically exhibit a linear slope $m_{ln}$ over $t$ and $t'$, respectively. However, our measurements show again solely curved behavior until large times (see Figure 7b).
To calculate $D_\pm^{ln}(c_0)$ the same method as for determining $D_\pm^{sqrt}(c_0)$ applies. We evaluate $\ln\left(\Delta\Phi_{long}^{relax}\right)$ and $\ln\left(\Delta\Phi_{long}^{charge} - U_{\bar{i}} - U_c\right)$ within the time interval during which the corresponding simulations yield linear behavior. Our 1D-model predicts linear behavior for $t = t' > 70$ s and $t = t' > 36$ s. For smaller times, the slope deviates for $> 5\%$.
The authors use again 20 s time segments to linearly fit the slope $m_{ln}$ of the curved relaxation data during the considered time interval. For fitting the linear behavior at large times we choose individual time intervals.
Due to the curvature, the slope yields again higher diffusion coefficients for time intervals including shorter

times. The time segments including the shortest times reveal the diffusion coefficients shown in Figure 7d. $D^{\ln}_{\pm}(c_0)$ exhibits an increasing trend for increasing concentration gradients $\Delta c$ at both temperatures. At 20 °C, the averaged diffusion coefficient for the highest current densities yields $(3.4 \pm 0.3) \cdot 10^{-10}\,\frac{\mathrm{m}^2}{\mathrm{s}}$. At 50 °C, $D^{\ln}_{\pm}(c_0)$ converges to a final value. Averaging $D^{\ln}_{\pm}(c_0)$ for $\Delta c > 10\,\mathrm{mM}$ results in $(4.7 \pm 0.4) \cdot 10^{-10}\,\frac{\mathrm{m}^2}{\mathrm{s}}$. These values are comparable to the literature.[1] The linear slope occurring at large $t$ results in similar diffusion coefficients for all current densities with $D^{\ln}_{\pm}(c_0) = (0.12 \pm 0.05) \cdot 10^{-10}\,\frac{\mathrm{m}^2}{\mathrm{s}}$ at 20 °C and $D^{\ln}_{\pm}(c_0) = (0.2 \pm 0.2) \cdot 10^{-10}\,\frac{\mathrm{m}^2}{\mathrm{s}}$ at 50 °C. These values are several times lower than reported in the literature.[1]

# 4. Very-Low-Frequency Impedance Spectroscopy

## 4.1. Non-Linearities

In the VLF-IS measurements, the authors apply elevated current density amplitudes to induce significantly high concentration gradients $\Delta c$. However, too high $\Delta c$ and overpotentials can induce non-linear effects. Therefore, we have to ensure that the linearized description of the system is still valid even for our highest current amplitudes. Our theory deviates if the Butler-Volmer equation reaches the non-linear regime and the current density $\bar{i}$ is no longer proportional to the overpotential $\eta_{\mathrm{lin}}$. Additionally, for induced high concentration gradients $\Delta c$ the approximation of the logarithmic term $\ln \frac{c+\delta c}{c-\delta c} \approx \frac{2\delta c}{c} = \frac{\Delta c}{c}$ is no longer valid and the electrolyte parameters become concentration-dependent. Therefore, we estimate the influence of the effects, using a 1-D model (see section 2.3). Unlike the theory in section 2.1.3, the model incorporates the empirical approximations of the concentration-dependent parameters from Landesfeind et al.[1] and the standard Butler-Volmer equation (see Eq. 28). Note, that we adjust the measured $TDF(c)$ values by a factor of 2 (see Section 2.3).

In the course of our experiments, the VLF-IS measurement with a current amplitude of 500 µA requires the highest overpotential $\eta$ and induces the largest concentration difference $\Delta c$ at 50 °C. Therefore, we compare the corresponding modeled impedance spectra to a linear reference with a tiny current amplitude $I_0 = 5\,\mu\mathrm{A}$. The modeled impedances incorporate data points for 30 frequencies between 0.1 Hz and 400 µHz, calculated with $\varepsilon = 0.55$, $\beta = 2.89$ and $R_{\mathrm{CT}} = 15\,\Omega$ (see black curve in Figure 8).

For the evaluation of the impedance data, an input current signal and its voltage response get Fourier-transformed. The ratio of the transformed complex data yields the impedance and its corresponding phase difference. Since the standard EIS measurement calculates this ratio only in the linear regime, higher harmonics of the response due to non-linearities are omitted. However, the non-linearities also affect the fundamental component of the signal and thus, still influence the impedance data.

Using the local electro-neutral model (see section 2.1.3) the resistance of bulk electrolyte $R_{\mathrm{el}}$ and charge transfer $R_{\mathrm{CT}}$ add up in an indistinguishable offset $R$ in the real-axis of the Nyquist plot. Therefore, the model resembles the impedance of a serial $R$-Ws equivalent circuit.

Applying elevated current densities on the cell induces high concentration gradients, especially for low frequencies. To isolate the non-linear influence of the logarithmic term the authors use the linearized

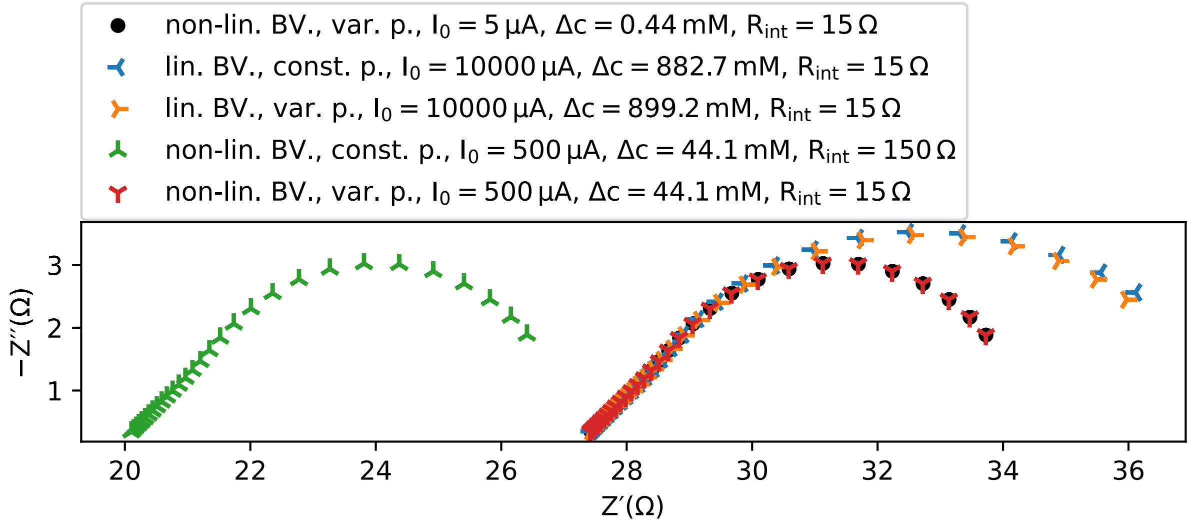


**Figure 8.** Modeled impedance spectra. The calculation with standard, non-linear Butler-Volmer equation (BV), varying electrolyte parameters (var. p.) and a small current amplitude $I_0 = 5\,\mu\mathrm{A}$ serves as a linear reference as the influence of the non-linearities is negligible. The same cell with $I_0 = 500\,\mu\mathrm{A}$ as used in our experiments shows the same results. Non-linear effects emerge either for higher charge transfer resistances $R_{\mathrm{CT}}$ or higher concentration gradients $\Delta c$.

Butler-Volmer equation and constant electrolyte parameters in our model. For our base concentration $c_0 = 0.5\,\mathrm{M}$, the linear approximation of the logarithmic term underestimates the chemical potential for concentration gradients $\Delta c < 0.173\,\mathrm{M}$ by <1%. Therefore, we calculate the galvanostatic steady-state concentration difference occurring in the impedance for low frequencies. At 20 °C, the maximum current amplitude $I_0 = 60\,\mu\mathrm{A}$ induces a concentration difference of $\Delta c = 0.0134\,\mathrm{M}$. At 50 °C, $I_0 = 500\,\mu\mathrm{A}$ leads to $\Delta c = 0.0441\,\mathrm{M}$. Thus, approximating the logarithmic term introduces a negligibly small error for our experiments. This is also confirmed by our modeled impedance spectrum with $I_0 = 500\,\mu\mathrm{A}$ at 50 °C, showing no significant deviations from the linear reference (see Figure 8).

Non-linear effects corresponding to the logarithmic expression emerge at higher $\Delta c$. To validate this, we model the impedance for a current amplitude of $I_0 = 10000\,\mu\mathrm{A}$. As expected, the impedance data shows for low frequencies higher values than the linear reference. Also, the phase is slightly affected (see blue curve in Figure 8).

This is due to the concentration difference $\Delta c$ being slightly shifted with respect to the current phase. Figure 9 shows the total cell voltage and its components, differentiated and subsequently normalized by the corresponding scaled linear cell voltage for the lowest frequency $f = 400\,\mu\mathrm{Hz}$. While the bulk and charge transfer potentials $U_{\mathrm{bulk}}$ and $U_{\mathrm{CT}}$ show no deviation the non-linear concentration potential $U_{\mathrm{conc}}$ reaches higher values than the linear, up-scaled one $U^{\mathrm{lin}}_{\mathrm{conc}}$. Thus, $U_{\mathrm{conc}}$ takes also a higher portion of the total cell potential $U_{\mathrm{tot}}$. Therefore, $U_{\mathrm{tot}}$ is increased and its phase is shifted towards the phase of $U_{\mathrm{conc}}$ (see blue curve in Figure 9).

Modeling the impedance using the concentration-dependent electrolyte parameters of Landesfeind et al. affects the whole behavior of the cell. Therefore, different concentration profiles are established at high induced concentration gradients due to varying diffusion coefficients and transference numbers (see Figure 10). For $I_0 = 60\,\mu\mathrm{A}$ and $I_0 = 500\,\mu\mathrm{A}$ and the corresponding maximum concentration difference $\Delta c = 0.0134\,\mathrm{M}$ and $\Delta c = 0.0441\,\mathrm{M}$, the deviation of the concentration-dependent parameters to the constant ones is below 1% and 2.5% at 20 °C and 50 °C. However, comparing the modeled concentration gradient $\Delta c$, potentials and impedance data using again a linear Butler-Volmer equation to the linear reference yields almost no difference.

The influence of varying electrolyte parameters becomes clear by calculating $\Delta c$ using $I_0 = 10000\,\mu\mathrm{A}$. Compared to constant parameters modeled with the same current amplitude, $\Delta c$ yields higher values. Together with the varying thermodynamic factor, this leads however to a smaller concentration potential difference $U_{\mathrm{conc}}$ and a slightly different phase. On the other hand, the concentration-dependent conductivity

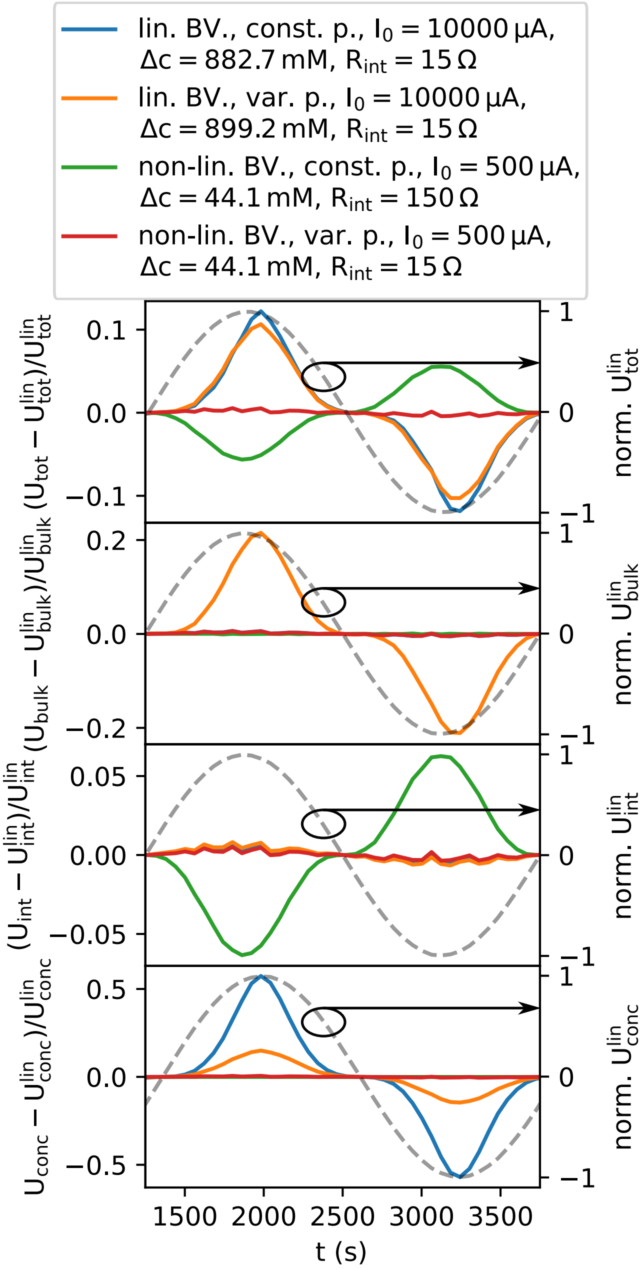


**Figure 9.** Normalized potential deviation between each the total potential $U_{\mathrm{tot}}$ response and its three components $U_{\mathrm{bulk}}$,$U_{\mathrm{CT}}$ and $U_{\mathrm{conc}}$, and the corresponding up-scaled linear potential for various simulation settings. While the simulation of our experiment with $I_0 = 500\mu\mathrm{A}$ shows no difference to the linear response, increasing the interface resistance from 15 Ω to 150 Ω introduces non-linear behavior in $U_{\mathrm{CT}}$ due to the Butler-Volmer equation. Increasing $I_0$ up to 10000 μA yields non-linear effects in $U_{\mathrm{conc}}$ for both constant and concentration-dependent electrolyte parameters. The latter additionally induces non-linear effects in $U_{\mathrm{bulk}}$.

$\kappa(c)$ increases the bulk potential $U_{\mathrm{bulk}}$ of the cell, leading to higher total cell potentials. Overall, $U_{\mathrm{tot}}$ is slightly decreased compared to constant electrolyte parameters, leading to a modified Nyquist plot for low frequencies (see orange curves in Figures 8 and 9).

Linearizing the Butler-Volmer equation overestimates the overpotential required for high current densities and thus overestimates the charge transfer resistance $R_{\mathrm{CT}}$. For galvanostatic impedance measurements, this

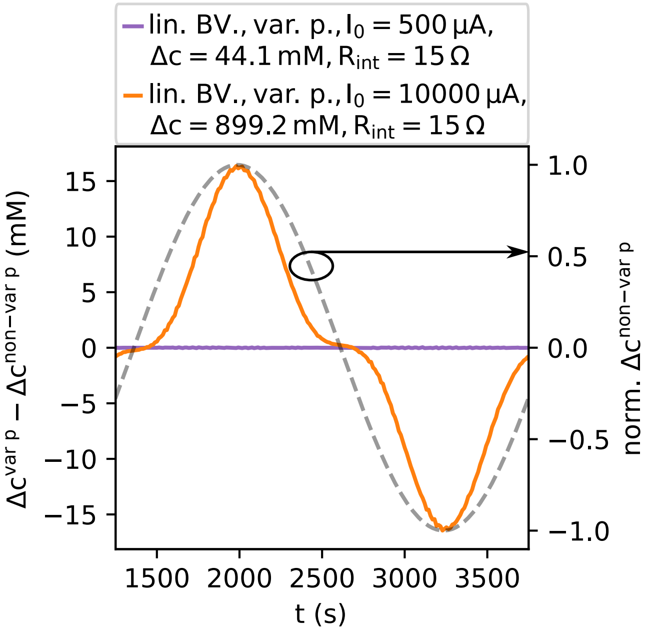


**Figure 10.** Deviation of the concentration difference $\Delta c$ due to concentration-dependent electrolyte parameters at $f = 400\,\mu Hz$. For the lower current amplitude $I_0 = 500\,\mu A$ as used in our experiments, the concentration difference yields the same values as for constant electrolyte parameters. For $I_0 = 10000\,\mu A$, $\Delta c$ reaches higher values than linearly expected.

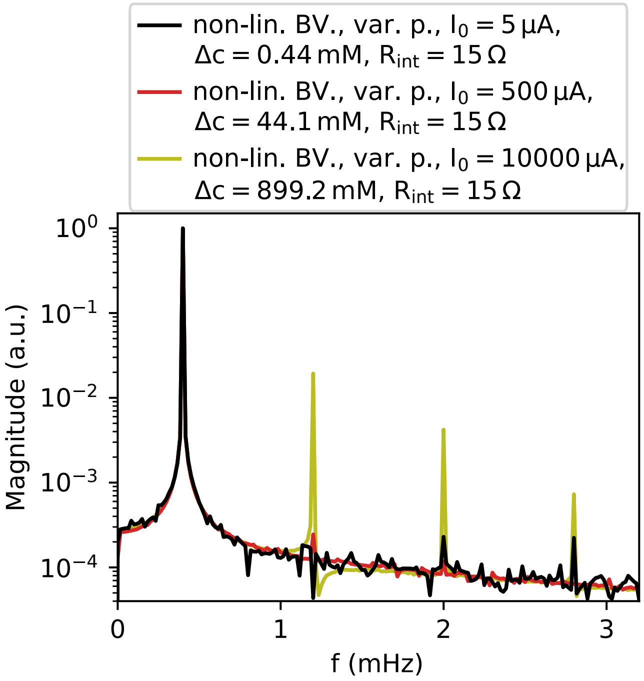


**Figure 11.** Normalized Fourier-transform of the potential response of the modeled linear reference with $I_0 = 5\,\mu A$, the simulation of our experiment with $I_0 = 500\,\mu A$ and an impedance with $I_0 = 10000\,\mu A$ at $f = 400\,\mu Hz$, using the standard Butler-Volmer equation and concentration-dependent electrolyte parameters. The transforms of linear response and experiment simulation show one main feature at $f = 400\,\mu Hz$ and only negligible contributions at higher harmonics. The transform of the potential response with $I_0 = 10000\,\mu A$ exhibits multiple features and therefore implies non-linear behavior.

is crucial for the peak values of the applied oscillating current density. Assuming a certain electrochemical potential the non-linear cell voltage is lower at these peaks than linearly expected. Therefore, also the impedance in the non-linear regime shifts to lower real values for all frequencies.

The overpotential deviation due to the linearization of the Butler-Volmer equation depends on the current density $\bar{\imath}$, the exchange current density $\bar{\imath}_0$ and thus on the charge transfer resistance $R_{CT}$. Considering the current amplitudes of $I_0 = 60\,\mu A$ and $I_0 = 500\,\mu A$ and a symmetry factor $\alpha = 0.5$ we calculate the maximal deviation to be below 1% for $\frac{R_{CT}}{2} < 208\,\Omega$ and $\frac{R_{CT}}{2} < 27.5\,\Omega$ for each electrode site. This yields a resistance of $R_{CT} < 416\,\Omega$ and $R_{CT} < 55\,\Omega$ for the total cell at 20 °C and 50 °C.

In the VLF-IS measurements, the charge transfer impedance is difficult to isolate since it overlaps with the impedance of the SEI. However, even the resistance of the combined impedances takes values below $R_{int} = 113\,\Omega$ and $R_{int} = 11\,\Omega$ for all measurements. Inserting even higher values $R_{CT} = 15\,\Omega$ in our $I_0 = 500\,\mu A$ impedance calculation does not yield significant deviations to the linear reference. Therefore, the linearisation of the Butler-Volmer is adequate for our experiments.

To demonstrate the non-linear effects of the Butler-Volmer equation, we increase the charge transfer resistance in our model to $R_{CT} = 150\,\Omega$ and repeat the impedance calculation, using constant electrolyte parameters. Subtracting $135\,\Omega$ of the resulting data allows a comparison to the linear reference. The resulting impedance data are shifted further to lower real values as expected for linear behavior.

Looking at the potential components, the cell with $R_{CT} = 150\,\Omega$ shows lower peak values of the charge transfer potential $U_{CT}$ compared to the up-scaled linear reference with $R_{CT} = 15\,\Omega$. This translates to also lower total cell voltages $U_{tot}$ and thus lower impedance values.

Since none of the discussed effects induces non-linear behavior in our experiments we summarize them in one impedance calculation, using the standard Butler-Volmer equation, varying electrolyte parameters with a current amplitude $I_0 = 500\,\mu A$. The result shows no difference to the linear reference in the Nyquist plot and the potentials (see red curve in Figures 8 and 9). This also shows in the normalized Fourier-transform of the potential response of the lowest frequency. In contrast to a current amplitude of $I_0 = 10000\,\mu A$, using $I_0 = 5\,\mu A$ and $I_0 = 500\,\mu A$ yields no significant contributions of higher harmonics (see Figure 11). Therefore, all non-linear effects seem to be negligibly small in our experiments.

Concentration-dependent electrolyte parameters also affect the concentration cell measurements of section 3.2. In this case, the concentration difference between the half-cells $\Delta c = 0.75\,M - 0.25\,M = 0.5\,M$ is very high. Therefore, the thermodynamic factors $TDF\,(0.75\,M)$, $TDF\,(0.25\,M)$ and the transference

numbers $t_+$ (0.75 M), $t_+$ (0.25 M) deviate strongly from their values at the base concentration $c_0 = 0.5$ M. The measured potential $U_{\text{conc}}$ is therefore up to 7% lower than linearly expected. Thus, also the determined factor $a(c_0)$ shifts to lower values.

## 4.2. Drift Correction

In our VLF-IS measurements, (see section 3.4) the authors detect the impedance data from 4 MHz down to 400 µHz. With three measuring periods and three steps per decade, the measurement has a duration of approximately 10 h. The detection of the high-frequency impedance data including the bulk resistance $R_{\text{el}}$ and the interface resistance $R_{\text{int}}$ lasts only a small fraction of the measuring time. Recording the low-frequency data points takes the main part of the measuring period. During this time the cell structure may however vary, for instance in terms of growing SEI or mossy Li structures on the electrode surface. This leads to a temporal modification of $R_{\text{int}}$. Therefore, the low-frequency data points do not only capture the diffusion effects but simultaneously the variation of $R_{\text{int}}$.
To compensate the influence of the variations in $R_{\text{int}}$, we correct the real part of the VLF-IS data. Note, that also the imaginary part may be influenced by the processes varying $R_{\text{int}}$. Since $R_{\text{int}}$ changes only slightly for the VLF-IS at 50 °C, the correction applies only to the impedance data for the measurements at 20 °C (see section 3.4). Similar procedures allow adding drifts to the fit-model of a VLF-IS measurement and observing its effect on the corresponding DRT (see SI section 4.5).
For the correction, we consider the determined values of $R_{\text{int}}$ for measurement $i$ and its subsequent measurement $i+1$. The difference between both values $\Delta R = R^{i+1}_{\text{int}} - R^{i}_{\text{int}}$ depicts the modification of $R_{\text{int}}$ occurring mainly during the detection of the low-frequency data points of measurement $i$. Assuming a linear modification of $R_{\text{int}}$ over time results in $R_{\text{int}}(t) = R_{\text{int}} + \Delta R \frac{t}{T}$. Here, $T$ specifies the total duration of the measurement. Depending on the point in time $t$ when each VLF-IS data point is recorded, the impedance is therefore shifted by $\Delta R \frac{t}{T}$ (see Figure 12).
Using the respective recording times $t$ we correct each impedance data point by $-\Delta R \frac{t}{T}$. Figure 13 shows exemplary the original VLF-IS data and its corresponding corrected values of the measurement with $I_0 = 10$ µA at 20 °C. While the high-frequency data points are unaffected the low-frequency data points are slightly shifted towards lower real values.

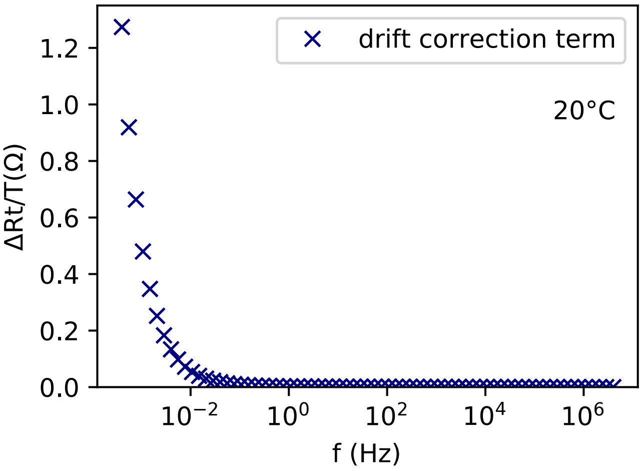


**Figure 12.** Drift correction term $\Delta R \frac{t}{T}$ over frequency. Assuming a linear drift of $R_{\text{int}}$ over time affects especially the low-frequency impedance data points.

## 4.3. Determination of $R_{\text{el}}$, $R_{\text{int}}$ and $\beta$

Using VLF-IS allows measuring the diffusive resistance $R_{\text{D}}$ of symmetrical Li metal | electrolyte + separator | Li metal cells. $R_{\text{D}}$ reveals convoluted information about the transference number $t_+(c_0)$ and the thermodynamic factor $TDF(c_0)$ in terms of factor $b(c_0)$ (see Eq. 25). Calculating $b(c_0)$ from $R_{\text{D}}$ requires knowledge about the morphological influence of the separator. Since $\varepsilon$ is stated by the manufacturer (see section2.2.3) the authors determine the Bruggemann-coefficient $\beta$. For this, we consider the high-frequency resistance revealing the bulk resistance $R_{\text{el}}$. Inserting $R_{\text{el}}$ in Eq. 23 yields $\beta$.
The fit results for $R_{\text{el}}$ over time are shown in Figure 14a. Note, that the applied current amplitude in the VLF-IS changes over time according to Table 2. $R_{\text{el}}$ takes values from 15.1 Ω to 19.8 Ω and 9.8 Ω to 13.7 Ω at 20 °C and 50 °C. At both temperatures, $R_{\text{el}}$ slowly increases for all cells except one cell at 20 °C. The resistance changes for less than 0.6 Ω and 1.5 Ω for each cell over the whole course of the respective experiments. Additionally, at 50 °C, $R_{\text{el}}$ shows a step-like decrease when the magnitude of the applied current amplitude increases. We attribute this effect to changes in the internal resistance of the measurement device. Averaging all results for 20 °C and 50 °C yields 17.7 Ω and 11.6 Ω. Together with the previously determined conductivities (see section 3.1), this leads to Bruggemann-coefficients $\beta = 3.1 \pm 0.3$ and $\beta = 2.9 \pm 0.3$ respectively. These values surpass the values obtained in the polarization experiments in section 3.3.
In order to track any changes to the interface between the Li electrode and the separator we also track the interface resistance $R_{\text{int}}$. At 20 °C, $R_{\text{int}}$ increases linearly over time starting from 73 Ω - 94 Ω up to 84 Ω - 114 Ω

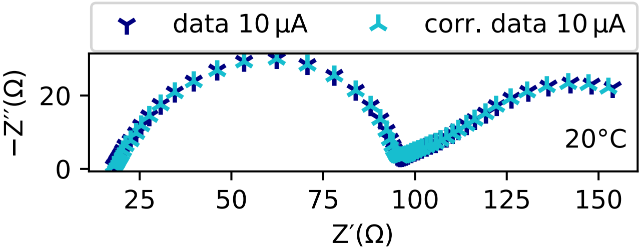


**Figure 13.** Original and corrected VLF-IS exemplary for a measurement with $I_0 = 10$ µA. The correction slightly shifts the real part of the low-frequency impedance to lower values.

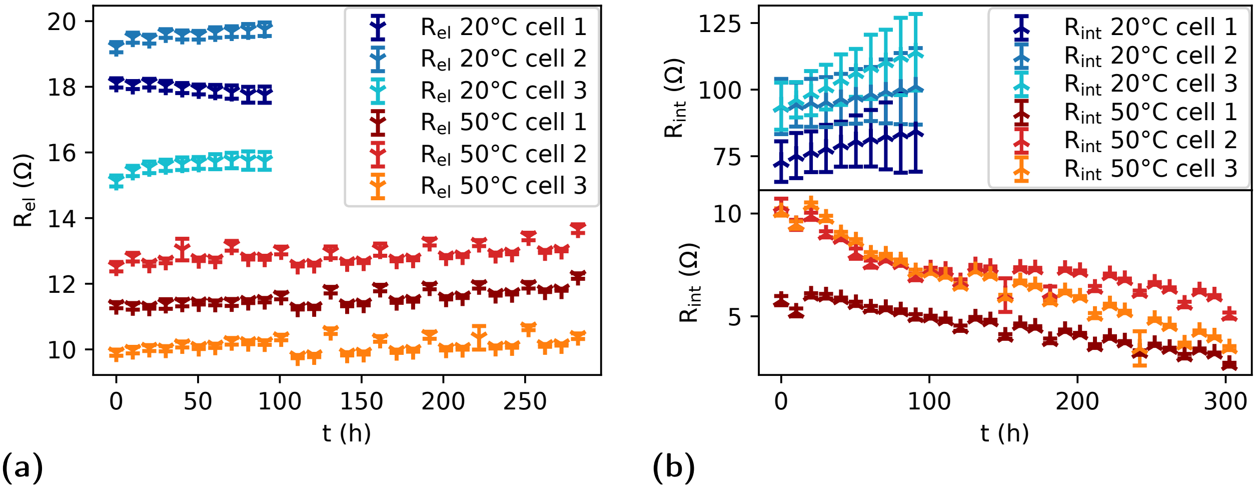


**Figure 14. a)** The bulk resistance $R_{\mathrm{el}}$ increases throughout the measurements except for one cell at 20 °C. This could hint towards growing dead mossy Li. **b)** The interfacial resistance $R_{\mathrm{int}}$ increases at 20 °C and decreases at 50 °C. This could be due to a growing SEI and growing live mossy Li respectively. The error bars represent the respective fit errors.

(see Figure 14b). Since this drift mostly affects the desired diffusion impedance it is removed as mentioned in section 4.2. At 50 °C, the resistance decreases - after an increase during the first VLF-IS conditioning cycles - from 6 Ω - 10 Ω down to 2.6 Ω - 5 Ω.

As mentioned in section 3.4, porous mossy Li on the pristine Li electrodes affects the impedance measurements.[6] According to Talian et al., the growth of dead mossy Li increases the bulk resistance $R_{\mathrm{el}}$. Thus, growing dead mossy Li could explain the increasing tendency of our measured $R_{\mathrm{el}}$ values in Figure 14a. Compared to the EIS measurements during the polarization measurements (see section 3.3), $R_{\mathrm{el}}$ takes elevated values in our VLF-IS experiments. This could be due to a higher amount of dead Li in the VLF-IS cells. However, also in the VLF-IS measurements, the increase of $R_{\mathrm{el}}$ does not correlate with the total transferred charge.

Increasing the coverage and thickness of the live mossy Li layer leads to an increasing active surface area of the electrode. This enhances the reaction kinetics, lowering the interface resistance $R_{\mathrm{int}}$. Opposed to this, a growing SEI increases $R_{\mathrm{int}}$. We therefore assign the increase of our measured $R_{\mathrm{int}}$ at 20 °C to SEI growth (see Figure 14b). At 50 °C, $R_{\mathrm{int}}$ decreases. This could originate from growing live mossy Li, overcompensating the effects of SEI growth. The phenomena measured with $R_{\mathrm{el}}$ and $R_{\mathrm{int}}$ hence both hint towards the growth of live and dead mossy Li.

## 4.4. Concentration Gradient Dependence of $R_{\mathrm{D}}^{\mathrm{tot}}$

Similar to the behavior of $R_{\mathrm{c}}$ in the galvanostatic polarization experiments (see section 3.3) the total diffusive resistance $R_{\mathrm{D}}^{\mathrm{tot}}$ in the VLF-IS decreases with increasing concentration gradients $\Delta c$ (see Figure 15). To ensure that the decrease of $R_{\mathrm{D}}^{\mathrm{tot}}$ is not only a time-dependent phenomenon we use the $I_0 = 10\,\mu\mathrm{A}$ reference impedance experiments at 50 °C. This allows tracking the temporal evolution of the total diffusive resistance. As Figure 15 indicates $R_{\mathrm{D}}^{\mathrm{tot}}$ is fairly stable in the reference measurements. Therefore, the resistance decrease can completely be attributed to increasing concentration gradients. This is consistent with the behavior of $R_{\mathrm{c}}$ in section 3.3.

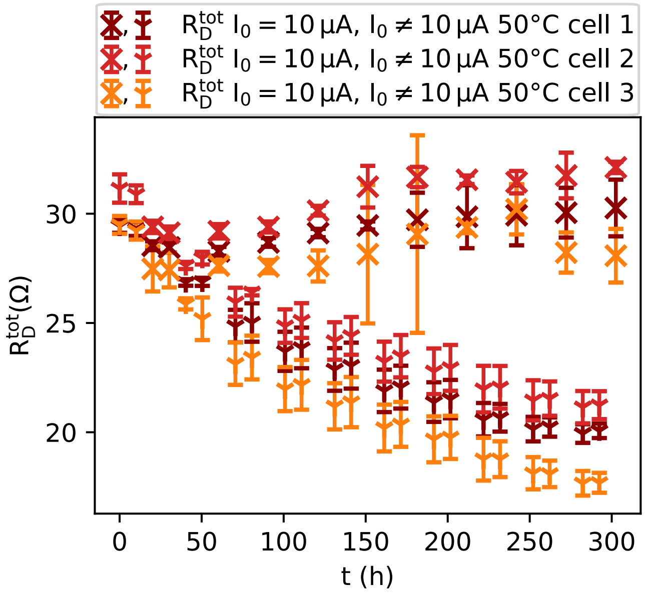


**Figure 15.** Total diffusive resistance $R_{\mathrm{D}}^{\mathrm{tot}}$ determined with various current amplitudes. The resistance decreases with increasing concentration gradient for both temperatures. At 50 °C, $R_{\mathrm{D}}^{\mathrm{tot}}$ converges to a final value. For $I_0 = 10\,\mu\mathrm{A}$, the resistance remains fairly stable over time. The error bars represent the respective fit error.

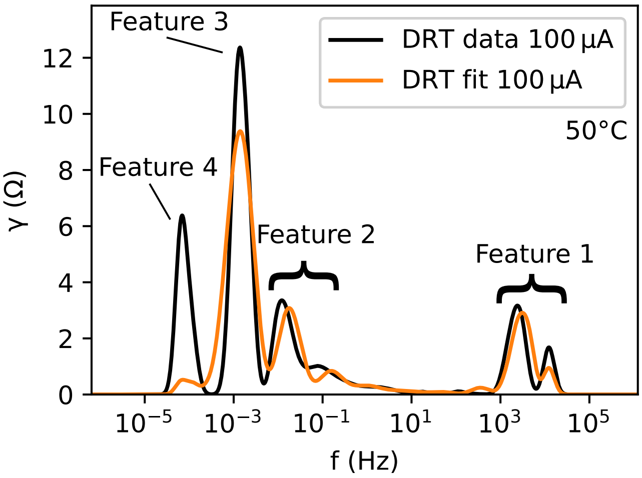


**Figure 16.** Comparison of the distribution of relaxation times (DRTs) of the impedance data and the corresponding fit-model. The DRTs deviate in feature 4 and the amplitude of feature 3.

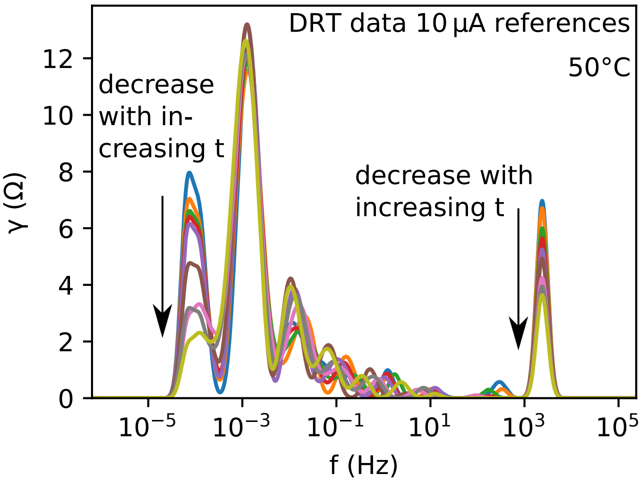


**Figure 17.** DRTs of the 10 µA reference measurements at 50 °C. Feature 1 and feature 4 decrease over time.

## 4.5. Distribution of Relaxation Times (DRT)

In section 3.4 the authors apply VLF-IS to symmetrical Li metal | electrolyte + separator | Li metal cells to measure the impedance of the diffusion processes through the separator. This reveals convoluted information about the transference number $t_+ (c_0)$ and the thermodynamic factor $TDF (c_0)$ in the form of factor $b (c_0)$ (see Eq. 25). Together with the specified factor $a (c_0)$ in section 3.2, Eqs. 7 and 8 allow deconvoluting these quantities. However, the impedance spectra show at least two overlapping features for low frequencies instead of one. Fitting the diffusive processes with two Warburg-short elements yields the corresponding amplitudes $R_\mathrm{D}$, deviating for both features from the theoretical expectations (see section 3.4). Therefore, we assume that additional diffusive processes through porous layers of mossy Li interfere with the diffusion through the separator.
In an attempt to identify the desired diffusion process, we calculate the distribution of relaxation times (DRT).[7–9] The DRT transforms the impedance data from the frequency into the time-domain. This yields a distribution of time constants corresponding to several serial RC-elements and provides a higher resolution of processes with similar resonance frequencies.
Comparing the DRT of the experimental data to the DRT of the corresponding fit-model may reveal deviations between both DRTs. These could hint towards additional processes which are not considered in the fit. We calculate the DRTs using the RelaxIS software (rhd instruments) with a regularization factor $\lambda = 10^{-4}$, a shape factor $s = 0.5$ and an interpolation factor $i = 100$. Since the DRTs are all quite similar, Figure 16 shows exemplary the DRT of a measurement with $I_0 = 100\,\mu\mathrm{A}$ at 50 °C over frequency.
The DRT of the measurements resembles the one of the fit. At high frequencies, both exhibit up to two peaks (feature 1). At lower frequencies, multiple peaks are visible (feature 2) followed by a high peak (feature 3). The amplitude of feature 3 in the DRT of the measurement exceeds the one of the DRT of the fit. Opposed to the fit, the DRT of the measurements shows at very low frequencies one additional peak (feature 4).
Due to their resonances, we assign the high-frequency peaks to interface effects $Z_\mathrm{int}$. The remaining features belong to diffusion effects considering their high time constants. In the Nyquist plots, Ws-elements represented the diffusion effects. In the DRT, these elements induce multiple peaks at higher frequencies next to the main peak.[9] The additional features can easily overlap with different processes impeding their deconvolution. This is probably the case for our VLF-IS measurements. Therefore, we assign feature 3 to $\mathrm{Ws}_2$. Its additional peaks overlap with the DRT of $\mathrm{Ws}_1$, generating feature 2. However, we cannot completely exclude further processes to be present in the frequency region of feature 2. Thus, feature 4 depicts the only candidate for a process that is not considered in the fit-model.
Considering the time evolution of the features mainly features 1 and 4 vary. Figure 17 shows this behavior exemplary for the 10 µA reference measurements at 50 °C. While the peak amplitude of feature 1 increases at 20 °C, it decreases over time at 50 °C. This corresponds to our findings of $R_\mathrm{int}$ in Figure 14b. Feature 4 shows similar behavior. However, especially the downward trend of this peak is peculiar since we do not expect disappearing diffusive effects over time and therefore doubt that this peak belongs to an additional diffusive process.
Noise and errors in the impedance data can heavily influence the DRT and even lead to artificial peaks.[8] In our VLF-IS measurements, the cells are slightly drifting since $R_\mathrm{int}$ changes (see Figure 14b). The drift especially affects the low-frequency impedance data and can impact the DRT. To show the influence of the drift, we consider three cases for the DRT of the fit-model. The first case is the DRT of the unmodified fit,

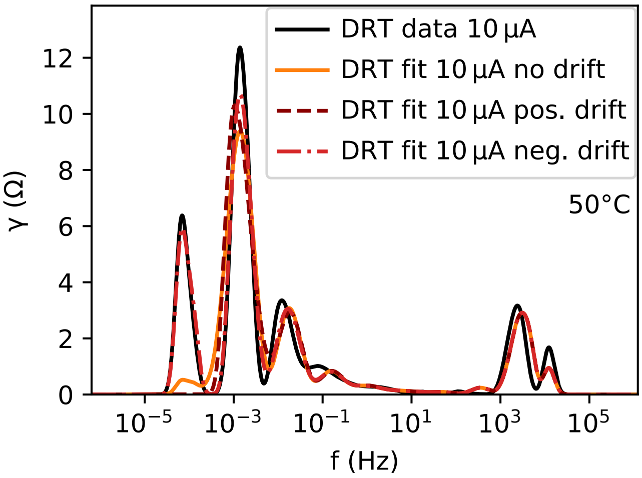


**Figure 18.** DRTs of the impedance data, the corresponding unmodified fit-model, and the fit-model with added positive and negative drifts. The drifts heavily influence the shape of the DRT. The negative drift adds an additional feature compared to the unmodified fit-model and resembles the DRT of the impedance data.

which has no drift. For the second and third case, we add a positive and negative temporally linear drift of 1 Ω in total to the real part of the fit. The procedure is similar to the drift correction in section 4.2. Figure 18 shows the corresponding DRTs. While a positive drift varies the resonance frequency and the peak height of feature 3, a negative drift also adds an additional low-frequency peak compared to the DRT without any drift (feature 4). This resembles the findings of the DRTs of the measurements well. Therefore, the decrease of $R_{\mathrm{int}}$ may induce the low-frequency peak at 50 °C. At 20 °C, we corrected the impedance data by a positive drift. However, possibly overcompensating the positive drift would also result in an overall negative drift. Therefore, we assign the low-frequency peak to the drift of the cells.

Even using the DRT, we can not resolve the diffusion through the separator from further processes. However, it should be noted that we expect the corresponding feature to be small. Also, the limited number of impedance data points makes the resolution process challenging.

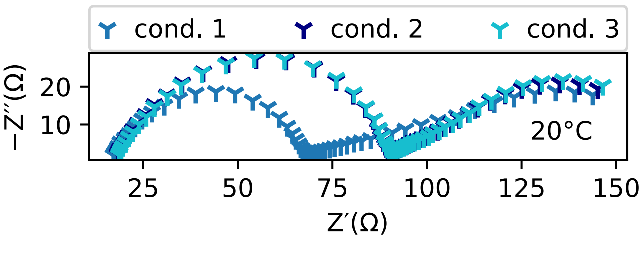


**Figure 19.** First three conditioning cycles at 20 °C. The diffusive resistance is already higher than expected after the second cycle.

## 4.6. Fast Growing Porous Layers on the Li Electrodes

The amplitude $R_{\mathrm{D}}$ of the diffusive impedance measured by VLF-IS exceeds the theoretical expectations. Therefore, the authors assume additional porous structures to be present on the Li metal surface (see section 3.4). The impedance data of the conditioning indicates that these structures have to form within the first conditioning cycle. The first conditioning cycle exhibits a large drift in the VLF-IS measurement. Subsequent conditioning cycles show rather stable behavior. However, the diffusive resistance is already very high $R_{\mathrm{D}}$ (see Figure 19). Therefore, we assume that the mossy Li already covers the surface area of the Li electrodes, even though our total transferred charge after the first cycle is tiny with $Q = 0.0186\,\frac{\mathrm{mAh}}{\mathrm{cm}^2}$. This corresponds to an approximately 12 nm thick Li-layer. However, the rapid sign change of the applied current densities could also form a porous mix of SEI and Li instead of the more structured layers described by Talian et al.[6]

## References


[1] J. Landesfeind, H. A. Gasteiger, *Journal of The Electrochemical Society* **2019**, *166*, A3079.

[2] J. Newman, K. Thomas-Alyea, *Electrochemical systems*, J. Wiley **2004**.

[3] A. Latz, J. Zausch, *Journal of Power Sources* **2011**, *196*, 3296.

[4] A. Latz, J. Zausch, *Beilstein Journal of Nanotechnology* **2015**, *6*, 987.

[5] J. Landesfeind, J. Hattendorff, A. Ehrl, W. A. Wall, H. A. Gasteiger, *Journal of The Electrochemical Society* **2016**, *163*, A1373.

[6] S. D. Talian, J. Bobnar, A. R. Sinigoj, I. Humar, M. Gaberšček, *The Journal of Physical Chemistry C* **2019**, *123*, 27997.

[7] H. Schichlein, A. Müller, M. Voigts, A. Krügel, E. Ivers-Tiffée, *Journal of Applied Electrochemistry* **2002**, *32*, 875.

[8] E. Ivers-Tiffée, A. Weber, *Journal of the Ceramic Society of Japan* **2017**, *125*, 193.

[9] M. A. Danzer, *Batteries* **2019**, *5*, 53.
